# Supplementary material for: Television Discourse Decoded: Comprehensive Multimodal Analytics at Scale
Source: arXiv:2402.12629 source file (2024-08-06)
Supplement: Supplementary file 1 [file dataset_related.tex]

\section{Dataset Curation}
\label{sec:dataset_appendix}
%\tableofcontents

%%%%%%%%%%%%%%%%%%%%%%%%%%%%%%%%%%%%%%%%%%%%%%%%%%%%%%%%%%%%%%%%
%%%%%%%%%%%%%%%%%%%%%%%%%%%%%%%%%%%%%%%%%%%%%%%%%%%%%%%%%%%%%%%%
%%%%%%%%%%%%%%%%%%%%%%%%%%%%%%%%%%%%%%%%%%%%%%%%%%%%%%%%%%%%%%%%
%%%%%%%%%%%%%%%%%%%%%%%%%%%%%%%%%%%%%%%%%%%%%%%%%%%%%%%%%%%%%%%%
%%%%%%%%%%%%%%%%%%%%%%%%%%%%%%%%%%%%%%%%%%%%%%%%%%%%%%%%%%%%%%%%
%\clearpage

\subsection{Tags}
The tags fell into 2 types: \textbf{(Type A)} Tags which provided valuable signals about the topic being discussed in the video such as `Sushant case CBI', `Pulwama grenade attack', `covishield vaccine'; and \textbf{(Type B)} Tags such as `exclusive', `breaking news', which were generic and unhelpful to comment on the topic being discussed in the video. Some examples of tags on videos are shown in Table \ref{tab:tags_example}.

\subsection{\textbf{Categorization of Videos}}

\textbf{Finding the Categories}: 
The debates are based on a variety of different topics such as Politics, Crime \& Justice, International Affairs etc. Economy etc., as has already been documented in \cite{caravan_article}. There are videos whose topic of discussion fell into multiple categories such as: the debate titled ``Can Congress Question Centre On Fuel Prices Anymore?'' is related to both the Economy but also has a political party involved in it. Moreover, we also wanted to capture whether a particular debate was ``Anti-Opposition'', ``Anti-ruling-party'' or ``Supporting-ruling-party'' in nature. To find the categories relevant to each debate, the following process was used:
\begin{itemize}
\item In order to utilize the tags present in the video metadata to map the videos to different categories, we mapped each tag $T$ to a category $C$ with the assumption that if a tag $T$ present in the tags of a video, then the video is likely to have content corresponding to category $C$. Tags of Type-B were simply filtered out whereas tags of type A were mapped to different categories. 
\item To make sure that each category has sufficient set of videos for analysis, we \textbf{merged some categories under a common umbrella category}. For eg: (1) The videos corresponding to `Sabarimala Case' and `Triple Talaq' were grouped under Religion. Likewise, the videos corresponding to `Regional Elections' and '2019 Elections' were grouped under Politics.
\item After using the above, we were still left with  $830$ videos to which no category was assigned as all their tags belonged to Type-B. However, the categories for some of these videos were easily identifiable using their title. To take advantage of this, we decided to use \textbf{OpenAI's ``gpt-3.5-turbo"} to assign categories for the videos based on their titles. The corresponding prompt can be found in \textbf{Table \ref{tab:namescategory_fetch_prompt}}.
\item The final set of categories assigned to the videos was a union of the categories obtained by (1) the tag-based-mapping and (2) prompting \textbf{OpenAI's ``gpt-3.5-turbo"}. 
\end{itemize}
%\include{tables_folder/simple_stats_table}
%%%%%%%%%%%%%%%%%%%%%%%%%%%%%%%%%%

%%%%%%%%%%%%%%%%%%%%%%%%%%%%%%%%%%%%%%%%%
\textbf{Segregating the categories into major and minor categories}: In order to account for granular aspects in the content of the debate, for each video, 2 sets of categories were assigned: \textbf{Major Category} which captured the main focus of the content discussed in the debate; and \textbf{Minor Categories} which were also discussed/represented in the video but were not the most-important focus. For each video, there can only be one major label i.e. it is a singleton. For example: A video (such as ``Donald Trump Praises Modi, Opposition Gets Heartburn" \footnote{\url{https://www.youtube.com/watch?v=y0U5r8AuE6w}}) can be related to International Affairs as the major label but can also depict the Opposition in a bad light. When a video had multiple categories assigned to it, the major category was assigned to be the one which came higher in the preference list shown in Table \ref{tab:category_priority_list} and the remaining categories were retained as minor category.

\begin{table}[ht!]
\centering
\caption{Priority List used to select the major category when a video was mapped to several categories}
\label{tab:category_priority_list}
\begin{tabular}{|p{\linewidth}|}
\hline
Ram Mandir Babri Masjid \\
Farmers Protest Issue \\
Citizenship Amendment Act \\
SSR Case \\
Pulwama-Balakot \\
Kashmir \\
COVID/Lockdown \\
Scam related to \channel \\
Scams \\
Russia-Ukraine \\
China \\
Pakistan \\
International Affairs \\
Economy \\
Supporting-ruling-party \\
Anti-Opposition \\
Anti-ruling-party \\
State level politics \\
Religion \\
Defense \& Terrorism \\
Education \\
Sports \\
Bollywood \\
Crime and Justice \\
Politics \\
Miscellaneous \\
\hline
\end{tabular}

\end{table}

\begin{table*}[htbp]
\centering
\caption{Table showing \underline{some} categories and a \underline{subset} of their corresponding mapped tags}
\label{tab:tag_category_mapping}
\begin{tabular}{|p{0.2\textwidth}|p{0.8\textwidth}|}
\hline
\textbf{Category} & \textbf{Tags} \\ \hline
China & Tiktok banned | Xi Jinping | Sonia Gandhi Xi Jinping deal | modi xi jinping | xi jinping in india | XI jinping in Mamallapuram | Bharat vs China | Boycott China | india china international news | india china border news | China clashes | China Tawang border dispute | Chinese Apps TikTok blocked | LAC dispute \\ \hline
%Triple Talaq & triple talaq debate | owaisi on triple talaq | triple talaq ordinance | arnab on triple talaq | triple talaq verdict | triple talaq banned \\ \hline
Ram Mandir Babri Masjid & babri masjid | ayodhya verdict | ram mandir ayodhya fight | subramanian swamy on ram mandir | tasleem rahmani on ayodhya | CBI Babri Masjid | ayodhya land settlement | Ayodhya case settlement | ram mandir 2025 | ayodhya march | cji impeachment linked to ayodhya | Ram Mandir politics | Ayodha mediation panel \\ \hline
%Sports & t20 world cup | icc t20 world cup 2022 | IPL | india backs ms dhoni | ms dhoni | indian football | indian football team | fifa banned india | RCB | MI | Virat Kohli Captaincy | arbaaz khan ipl betting case | ipl betting scandal \\ \hline
Covid & China virus | Covishield | Vaccine in India | covishield | rahul gandhi questions vaccine | Is Covishield safe | Vaccine registration | 21 day lockdown | lockdown extension | coronavirus disease | covid china | covid origin | corona in india social media | pm modi on covid vaccine | lockdown violators | Coronavirus India lockdown | lockdown 21 day | 21 days lockdown | Modi coronavirus lockdown | Coronavirus warriors attacked \\ \hline
Pulawama Balakot & major gaurav arya on pulwama | pulwama terror attack | surgical strike | gen gd bakshi on surgical strike | Pulwama attack | avenge pulwama | pm modi on surgical strike | Surgical Strike \\ \hline
Farmers Protest & farmer protest | Farmer Bill 2020 | govt farmer talks | Centre Farmer talks | Farm Bill 2020 | Farm Bills explained | Three Farm Bills | sc hearing on farm law | haryana farmers protest live | haryana farmers protest latest | haryana farmers protest study iq | haryana farmers protest lallantop \\ \hline
Bollywood & Deepika Padukone | Sara Ali Khan | bollywood drug party | kangana ranaut interview | ncb summons bollywood | Aryan Khan drugs case | richa chadha on indian army | me too campaign \\ \hline
Issues related to \channel~ such as TRP Scam issue & Param Bir Singh case | fake trp | Param Bir Sachin Vaze secret meet | Sadhvi Pragya exposes Param Bir Singh | cbi fir trp scam case | arnab goswami trp scam | trp scam cbi | Param Bir Extortion racket\\ \hline
Economy & budget 2019 | nirmala sitharaman budget | union budget 2022 highlights | PM modi Economy push | rahul gandhi on fuel price | demonetization india | pm modi on fuel prices | arun jaitley gst | Make in India \\ \hline
%Regional Elections & tamil nadu election | tamil nadu election 2021 | tamil nadu politics | tamil nadu assembly election 2021 | Tamil Nadu 2021 2021 elections | gujarat elections | UP elections | Uttar Pradesh Polls | UP polls 2022 \\ \hline
2019 Elections & elections 2019 | 2019 lok sabha elections | who will win 2019 | election opinion poll 2019 | modi back in 2019 | modi sweep back in 2019 | manifesto 2019 | rahul gandhi 2019 manifesto | 2019 election survey | third front 2019 | bjp vs congress 2019 \\ \hline
Sabarimala Case & Politics on Sabarimala | sabarimala updates | sabarimala temple issue | womens entry in sabarimala | sabarimala verdict supreme court | trupti desai on sabarimala | rahul easwar sabarimala debate | sabarimala protest pandalam \\ \hline
\end{tabular}
\end{table*}

\begin{table*}[h]
\caption{Prompt fed to LLAMA-2-13b-chat to fetch names from the transcriptGPT-3.5-Turbo to fetch the categories for the videos}
\label{tab:namescategory_fetch_prompt}
\begin{tabularx}{\linewidth}{|>{\raggedright\arraybackslash}X|}
\hline
Please map the below debate titles for debates conducted on an Indian news channel into different topics based on the title of the debates. One debate may belong to multiple topics. \\\\

\textbf{List of topics}:- [Politics, \sensitive{Supporting-BJP, Anti-BJP}, Anti-Opposition, State level politics, Scams, Religion, Economy, Defense \& Terrorism, International Affairs, COVID/Lockdown, Bollywood, Farmers Protest Issue, Ram Mandir Babri Masjid, Citizenship Amendment Act, Kashmir, Pakistan, Pulwama-Balakot, Crime and Justice, Sports, Education] \\

\textbf{Here is some additional context about topics:-} \\

- \sensitive{Supporting-BJP}: Debate titles that shows positive bias against BJP or BJP affiliated leaders. Eg: Why The Yogi Victory Is Historic 2022 Election Results. \\

- \sensitive{Anti-BJP}: Debate titles that shows negative bias against BJP or BJP affiliated leaders. Eg: Shouldn't UP CM Yogi Adityanath Rise Above Namecalling, Barbaric Cruelty' Allegation Against Seema Patra - BJP Suspends But No Arrest,Is Modi Wave On The Wane. \\

- Anti-Opposition: Debate titles that shows negative bias against Opposition such as Congress or criticisms about the Opposition affiliated leaders like Vadra and Gandhis. Eg: Will Priyanka Vadra Take Responsibility For Stampede At Children's Rally, PM Modi Sets Vision For 2047, Will Opposition Rise Above Petty Politics. \\

- Politics: Debates including day-to-day political developments with no broader themes and political debates with no clear bias in the title. Eg: Centre Launches 'Agnipath' For India - Is It A Gamechanger Or Not, Kharge Compares PM Modi To 'Ravan'. Will The Insult Politics Backfire \\

- State level politics: Debate titles with any mention of an Indian state or a state leader. Eg: Eknath Shinde Stakes Claim On Shiv Sena, Is MVA Govt's Time Up,Sanjay Raut Abuses Shinde Camp; Uddhav Thackeray Extends Olive Branch To Rebels, Tamil Nadu BJP Chief K Annamalai Speaks To Arnab, Threatens 'Mass Satyagraha' Over Fuel Price. \\\\

For each debate title and id, perform the following actions: \\
1 - Read the debate title \\
2 - Iterate through all topics in above list of topics and determine whether topic is relevant to the debate \\
3 - Keep track of all relevant topics to the debate. Note that some of the debates may be relevant to multiple topics. In such cases, include all the topics relevant. \\
Separate responses for separate debates with a newline. Provide them in JSON format with the following keys: \\
- debate\_id: \textless debate ID\textgreater, \\
- debate\_title: \textless debate title\textgreater, \\
- topics\_list: \textless list of topics mapped to\textgreater, \\
- reasoning: \textless Reasoning behind mapping\textgreater \\
\\
\textbf{Debate titles list (each debate on a new line with format: \textless debate ID\textgreater | \textless debate title\textgreater):} \\
AM4jNtwHX8k | Did Rahul Gandhi Link PM Modi To "Hindu Terror" \\
UK4WtrqwD1U | PM Modi Sold 'Chai' \& Not The Nation \\
a2GaKNHfLz0 | BIGGEST EXPOSE: Church Campaign Against Nationalism \\
lk-pPzP8K2g | Woman Misses Funeral Due To VVIP Racism \\
lbliEqB27nY | Rahul Gandhi To Lead The Congress Party \\
\hline
\end{tabularx}
\end{table*}

\begin{table*}[h]
\caption{Prompt fed to LLAMA-2-13b-chat to fetch names from the transcript}
\label{tab:names_fetch_prompt}
\begin{tabularx}{\linewidth}{|>{\raggedright\arraybackslash}X|}
\hline
%%%%%%%%%%%%%%%%%%%%%%%%%%%%%%%%%%%%%%
\textless s\textgreater[INST] \textless\textless SYS\textgreater\textgreater\\You are a helpful, respectful and honest assistant. Always answer as helpfully as possible, while being safe.  Your answers should not include any harmful, unethical, racist, sexist, toxic, dangerous, or illegal content. Please ensure that your responses are socially unbiased and positive in nature.\\\\If a question does not make any sense, or is not factually coherent, explain why instead of answering something not correct. If you don't know the answer to a question, please don't share false information.\\\textless\textless SYS\textgreater\textgreater\\ \textit{Below within backticks is the transcript from a TV debate in India.    Extract the names of the speakers and panel members from the transcript.    HINT: the speakers are generally introduced in the beginning of the transcript by the debate moderator. Try using this introductory statement to find the names.     NOTE: Output the names as with numbering on new lines. In case the transcript has foul language, ignore the inappropriate language and personal attacks and focus only on finding the names.}    \\\\ \textbf{Transcript:} \\```\sensitive{Mumbai Studios of Republic TV. It's time for Arnab Goswami on the debate}. \\ \textbf{\textless speaker change\textgreater}\\  Good evening and welcome viewers. I don't believe in coincidences. The CBI director hates his number two and is fighting to stop him from taking over when he retires in a few weeks. The lawyer Prashant Bhushan steps in and challenges the appointment of the number two in the Supreme Court. 

This means that the CBI director obviously loves this and would love what Prashant Bhushan is doing for him. The CBI director then meets Prashant Bhushan and two people denied a birth in the Modi government. The permanently sulking Yashwant Sinha and Arun Shourie and Rafal. Viewers I'm asking you this, is this a coincidence? 

I may not name them viewers but now we all know who the lobby is. The lobby wants to engineer trouble within our country. Caste wars, they failed. Breaking down the Supreme Court, they failed. Dividing the Hindu religion, they failed. Destroying the agencies from within, they are trying. They will fail. It is our fundamental duty viewers, yours and mine, to make sure that they fail this time as well. We have to fight the lobby.

\textbf{\textless speaker change\textgreater}

....

\textbf{\textless speaker change\textgreater}
And if you will permit, Arnab this is basically, Arnab is, they tried it here, now they have hatched out to the CBI, hatched out to IP, for his role in the Godhra investigation, or his role, his question, his role in Gujarat came under huge question, his role in the Godhra investigation, his role in the Amit Shah case, so and then to bring him here, Mr. Modi lost the plot, he thinks, he thought he could run everything, but he can't, he has complete control of governance, of policy, they don't know the government can't do any policy, so please do not bring in this whole thing about casting us questions, if it's to our five investigative agents, in which we have been saying all the time, we are not even talking about policy, which they don't understand a word, but this is simple administrative issue.```
\\

[\slash INST]

\\\hline

\end{tabularx}

\end{table*}

\subsection{Annotation Methodology}
\label{sec:annotation_guidelines}

\subsubsection{Objective}

Annotate whether the major and minor category labels per video are correct or not.

To annotate a video, the main focus would be the Title and hashtags provided in the sheet. If the signals aren’t sufficient then proceed to check the video’s first 5 minutes where the news anchor gives the synopsis of the debate. Keep watching video at a lower priority since annotation time might increase.

\subsubsection{For Major Category}
\textit{Below is the list of major categories that you will find during annotation. They are ordered from specific to more generic labels.}\\
So for example, if the video talks about the CAA act and is political in nature, give preference to the CAA label since it is more specific. Politics will be part of the minor label.
\textbf{If you feel the major label assigned is incorrect then mark the cell in red and add an additional comment providing the suitable category you think should be present.}

%\clearpage

\subsubsection{Fuzzy matching and clustering names}
\label{sec:appendix_names}
While within the transcript of a video, the LLM was fairly robust to errors, we found that across different videos, there was still some variation in name for the same individual. We started with a seed set of most frequently occurring names (representing one cluster each) and iterated through all others names to see whether there was a fuzzy match for any of the names in the seed set. If a name was not a close match to any of the names in the seed set, the name was added as a new cluster to the seed set; else it was added to the cluster of the name it was fuzzy matched to. This also helped expand our seed set. We used a combination of 2 matching algorithms: (1) ``Partial Token Sort Ratio'' \cite{fuzzy_match_lib} (which helped match names where one name had more tokens than the other, eg: general bakshi, major general gd bakshi), (2) metaphone based matching (which helped match names which had the same pronunciation but different spellings, eg: ``syed asad abbas'', ``sayyad asad abbas'', ``sayyed asad abbas'', ``syed assad abbas'' all of which have the same metaphone: ``SYT AST ABS'').

\subsection{Bias in transcripts}

%%%%%%%%%%%%%%%%%%%%%%%%%%%%%%%%%%%

Table \ref{classifier_dataset_keywords} shows the list of keywords we used containing politicians and political parties.\\
Table \ref{tab:negation_keywords} shows the list of negation words.\\
Table~\ref{tab:bjp_ig} shows the full list of keywords.

\subsection{More plots related to Incivility, Overlap, Foul and gender bias}

Figures~\ref{fig:incivility_all},~\ref{fig:toxic_all} show additional plots for all incivility.

\begin{table*}[!htb]
    \caption{\textbf{One-Tailed \textit{t}-test for the hypotheses $H_{M,greater}$ and $H_{M,lesser}$, we report \textit{t}-stat for $\alpha=$ 0.01}}
    \label{tab:hypo_incivility}
    \begin{subtable}{.5\linewidth}
      \centering

      \caption{One-Tailed t-test for $H_{M,greater}$}
      \label{tab:hypo_greater}
     {\small
\begin{tabular}{@{}p{1.75cm}@{\hspace{4pt}}ccccc@{}}
    \toprule
    \textbf{Category $M$} & \textbf{$Mean($M$)$} & \textbf{$Mean(Rest)$} & \textbf{\textit{t}-stat} & \textbf{\textit{p}-value}\\
    \midrule
    CAA & 0.2157 & 0.1598 & 5.684 & 7.255e-09 \\
    Kashmir & 0.1947 & 0.1593 & 5.065 & 2.176e-07 \\
    Politics & 0.1829 & 0.1477 & 10.397 & 3.644e-25 \\
    Pulwama-Balakot & 0.2500 & 0.1601 & 6.561 & 3.175e-11 \\
    Religion & 0.1959 & 0.1584 & 6.146 & 4.551e-10 \\
    \bottomrule
\end{tabular}
}
    \end{subtable}%
    \begin{subtable}{.5\linewidth}
      \centering

      \caption{One-Tailed t-test for $H_{M,lesser}$}
      \label{tab:hypo_lesser}
      {\small
\begin{tabular}{@{}p{2.5cm}@{\hspace{5pt}}ccccc@{}}
    \toprule
    \textbf{Category $M$} & \textbf{$Mean($M$)$} & \textbf{$Mean(Rest)$} & \textbf{\textit{t}-stat} & \textbf{\textit{p}-value}\\
    \midrule
    COVID/Lockdown & 0.0710 & 0.1670 & -13.804 & 2.804e-42 \\
    TRP Scam related to \channel & 0.0715 & 0.1636 & -8.362 & 4.796e-17 \\
    %Crime and Justice & 0.1502 & 0.1622 & -1.752 & 0.0400 \\
    International Affairs & 0.1136 & 0.1645 & -7.252 & 2.655e-13 \\
    %Farmers Protest Issue & 0.1372 & 0.1618 & -1.647 & 0.0499 \\
    China & 0.0962 & 0.1628 & -5.581 & 1.311e-08 \\
    Sports & 0.0940 & 0.1621 & -3.975 & 3.602e-05 \\
    Bollywood & 0.1185 & 0.1636 & -5.696 & 6.761e-09 \\
    \bottomrule
\end{tabular}
}
    \end{subtable} 
\end{table*}

\begin{table*}[!htb]
    \caption{\textbf{One-Tailed \textit{t}-test for the hypotheses that difference between distribution of overlap speech and toxicity between \channel vs other shows is statistically significant, we report \textit{t}-stat for $\alpha=$ 0.05}}
    \label{tab:hypo_incivility_other_debates}
    \begin{subtable}{.5\linewidth}
      \centering

      \caption{Two-Tailed t-test for Overlap Speech}
      \label{tab:hypo_overlap_other_debates}
     {\small
\begin{tabular}{@{}p{2.5cm}@{\hspace{5pt}}ccccc@{}}
    \toprule
    \textbf{Debate} & \textbf{$Mean(TV Debates)$} & \textbf{\textit{t}-stat} & \textbf{\textit{p}-value}\\
    \midrule
    	\channel & 0.1448 & NA & NA \\
	France 24 & 0.0076 & 23.2468 & 5.98-110 \\
	Sky News UK & 0.0984 & 5.1663 & 2.55-07 \\
	US Presidential Elections & 0.0175 & 9.9175 & 8.21-23 \\
	Morning show with Joe & 0.0069 & 35.2401 & 4.41-230 \\
    \bottomrule
\end{tabular}
}
    \end{subtable}%
    \begin{subtable}{.5\linewidth}
      \centering

      \caption{Two-Tailed t-test for Toxicity}
      \label{tab:hypo_toxic_other_debates}
      {\small
\begin{tabular}{@{}p{2.5cm}@{\hspace{5pt}}ccccc@{}}
    \toprule
    \textbf{Debate} & \textbf{$Mean(TV Debates)$} & \textbf{\textit{t}-stat} & \textbf{\textit{p}-value}\\
    \midrule
	\channel & 0.0166 & NA & NA \\
	France 24 & 0.0021 & 6.9221 & 5.43-12 \\
	Sky News UK & 0.0110 & 1.7640 & 0.0778 \\
	US Presidential Elections & 0.0053 & 2.4801 & 0.01 \\
	Morning show with Joe & 0.0081 & 5.9825 & 2.44-09 \\
    \bottomrule
\end{tabular}
}
    \end{subtable} 
\end{table*}

%%%%%%%%%%%%%%%%%%%%%%%%%%%%%%%%%%%%%%%%
\begin{table*}[htbp]
\centering
\captionsetup{width=\linewidth}
\caption{Few examples of tags associated with the various videos}
\label{tab:tags_example}
\begin{tabularx}{\linewidth}{|>{\hsize=0.3\hsize}X|>{\hsize=0.7\hsize}X|}
\hline
\textbf{Title} & \textbf{Tags} \\
\hline
\href{https://www.youtube.com/watch?v=ec9X8bC96Eo}{CBI To Probe 'Witness Coercion' Tapes, Param Bir In Deep Trouble} & CBI TRP case, Witness tapes, TRP case manipulation, TRP witness scam, TRP witness coercion tapes, india today trp scam, republic tv fake trp, india today fake trp \\
\hline
\href{https://www.youtube.com/watch?v=Mdj3BrofgUI}{Justice For Sushant: Demand Grows For CBI Investigation} & Sushant Singh rajput, Sushant Singh Rajput soul talks, Sushant Singh Rajput murdered by Suraj Pancholi, Rumi Jaffery, Mumbai Police Sushant Singh,Sushant Singh Rajput spirit calling, Kangana Ranaut, Kangana Ranaut Sushant Singh, Kangana Ranaut \\
\hline
\href{https://www.youtube.com/watch?v=PRrQCwnrH0Y}{Jyotiraditya Scindia's Exit Stings Congress} & Sonia Gandhi, Rahul Gandhi, maharashtra politics, maharashtra government, maha vikas aghadi rift, NCP, Shiv sena, uddhav thackeray, sharad Pawar, Priyanka Gandhi, Scinida, jyotiraditya scindia, jyotiraditya scindia bjp join,  jyotiraditya scindia quits congress \\
\hline
\href{https://www.youtube.com/watch?v=-jU1IBxhGrU}{Nation backs MS Dhoni Wearing The `Balidaan Badge'} & indian premier league, Balidaan Badge, balidaan badge controversy, glove controversy, india backs ms dhoni, national pride, balidan badge indian army, ms dhoni, world cup 2019 indian team, bcci, indian cricket team, 2019 world cup indian team, bcci writes to ICC \\
\hline
\href{https://www.youtube.com/watch?v=Oy3aJ18FMoY}{Will Yogi Adityanath Sack Rape Accused MLA?} & cm yogi adityanath, unnao rape case, kuldeep singh sengar, bjp mla rape case, mla rape case, rape victim father death, cbi investigation of unnao, uttar pradesh, unnao case, bjp mla brother arrested, up police on unnao, cm yogi on unnao case \\
\hline
\end{tabularx}
\end{table*}
%%%%%%%%%%%%%%%%%%%%%%%%%%%%%

\begin{table}[htbp]
    \centering
    \caption{Negation Words}
    \label{tab:negation_keywords}
    \begin{tabular}{|p{1\columnwidth}|}
        \hline
        not, don’t, can’t, won’t, shouldn’t, mustn’t, should not, must not, do not, cannot, will not, would not, wouldn’t, isn’t, is not, dare not, have not, might not, may not, need not, ought not, shall not \\
        \hline
    \end{tabular}
\end{table}

% \begin{table}[htbp]
%     \centering
%     \caption{Negation Words}
%     \label{tab:negation_keywords}
%     \begin{tabular}{|c|}
%         \hline
%         not, don't, can't, won't, shouldn't, mustn't, should not, must not, do not, cannot, will not, would not, wouldn't, isn't, is not, dare not, have not, might not, may not, need not, ought not, shall not \\
%         \hline
%     \end{tabular}
% \end{table}

\subsection{Hashtag Bias}
Table \ref{tab:hashtag_bias} shows the bias in the use of hashtags. These hashtags were extracted from the videos using OCR.

% \input{tables_folder/hashtag_bais}
% \begin{table}[ht]
%     \centering
%     \caption{Hashtags showcasing the level of scrutiny between videos in Anti-BJP vs Anti-Opposition videos}
%     \label{tab:hashtag_bias}
%     \begin{tabular}{|p{0.45\columnwidth}|p{0.45\columnwidth}|}
%         \hline
%         \textbf{Hashtags used in Anti-BJP videos} & \textbf{Hashtags used in Anti-Opposition videos}\\
%         \hline
%         BaggaTweetArrest, YogiWakesUp, GovernorRightorWrong, ItalyKeSaudagar, WillYogiSackMLA, YogiWakeUp, FightForAsifa, SadhviBackGodse, SackBJPBrat, RepublicVsBJPMLA, YogicopsStung, NetasChokeDelhi, BJPWakeUpCall & CongRapeComment, SoniaSainik, MayaDumpsCong, CongPoliticsofAbuse, CongVsCitizens, ConginsultsDemocracy, ECBansMamata, MamataLosesGrip, AAPForFreebies, CongFallsApart, KejriwalMinisterArrested, NeechPolitics, VadraCongChaos, CongRajCollapse, VadrasMustGo, RahulMocksForces, CongresslIsOver, RahulGetsDumped, CongAbusesRashtrapati, RahulCheatsPoor
% \\
%         \hline
%     \end{tabular}

% \end{table}

\begin{table}[ht]
    \centering
    \caption{Hashtags showcasing the level of scrutiny between videos in Anti-ruling-party vs Anti-Opposition videos}
    \label{tab:hashtag_bias} % Place the \label command here
    \begin{tabular}{|p{0.35\columnwidth}|p{0.55\columnwidth}|}
        \hline
        \textbf{Hashtags used in Anti-ruling-party videos} & \textbf{Hashtags used in Anti-Opposition videos}\\
        \hline
        BaggaTweetArrest, YogiWakesUp, GovernorRightorWrong, ItalyKeSaudagar, WillYogiSackMLA, YogiWakeUp, FightForAsifa, SadhviBackGodse, SackBJPBrat, RepublicVsBJPMLA, YogicopsStung, NetasChokeDelhi, BJPWakeUpCall & CongRapeComment, SoniaSainik, MayaDumpsCong, CongPoliticsofAbuse, CongVsCitizens, ConginsultsDemocracy, ECBansMamata, MamataLosesGrip, AAPForFreebies, CongFallsApart, KejriwalMinisterArrested, NeechPolitics, VadraCongChaos, CongRajCollapse, VadrasMustGo, RahulMocksForces, CongresslIsOver, RahulGetsDumped, CongAbusesRashtrapati, RahulCheatsPoor
\\
        \hline
    \end{tabular}
\end{table}

\begin{figure*}[htbp]
  \centering
  \includegraphics[width=1\linewidth]{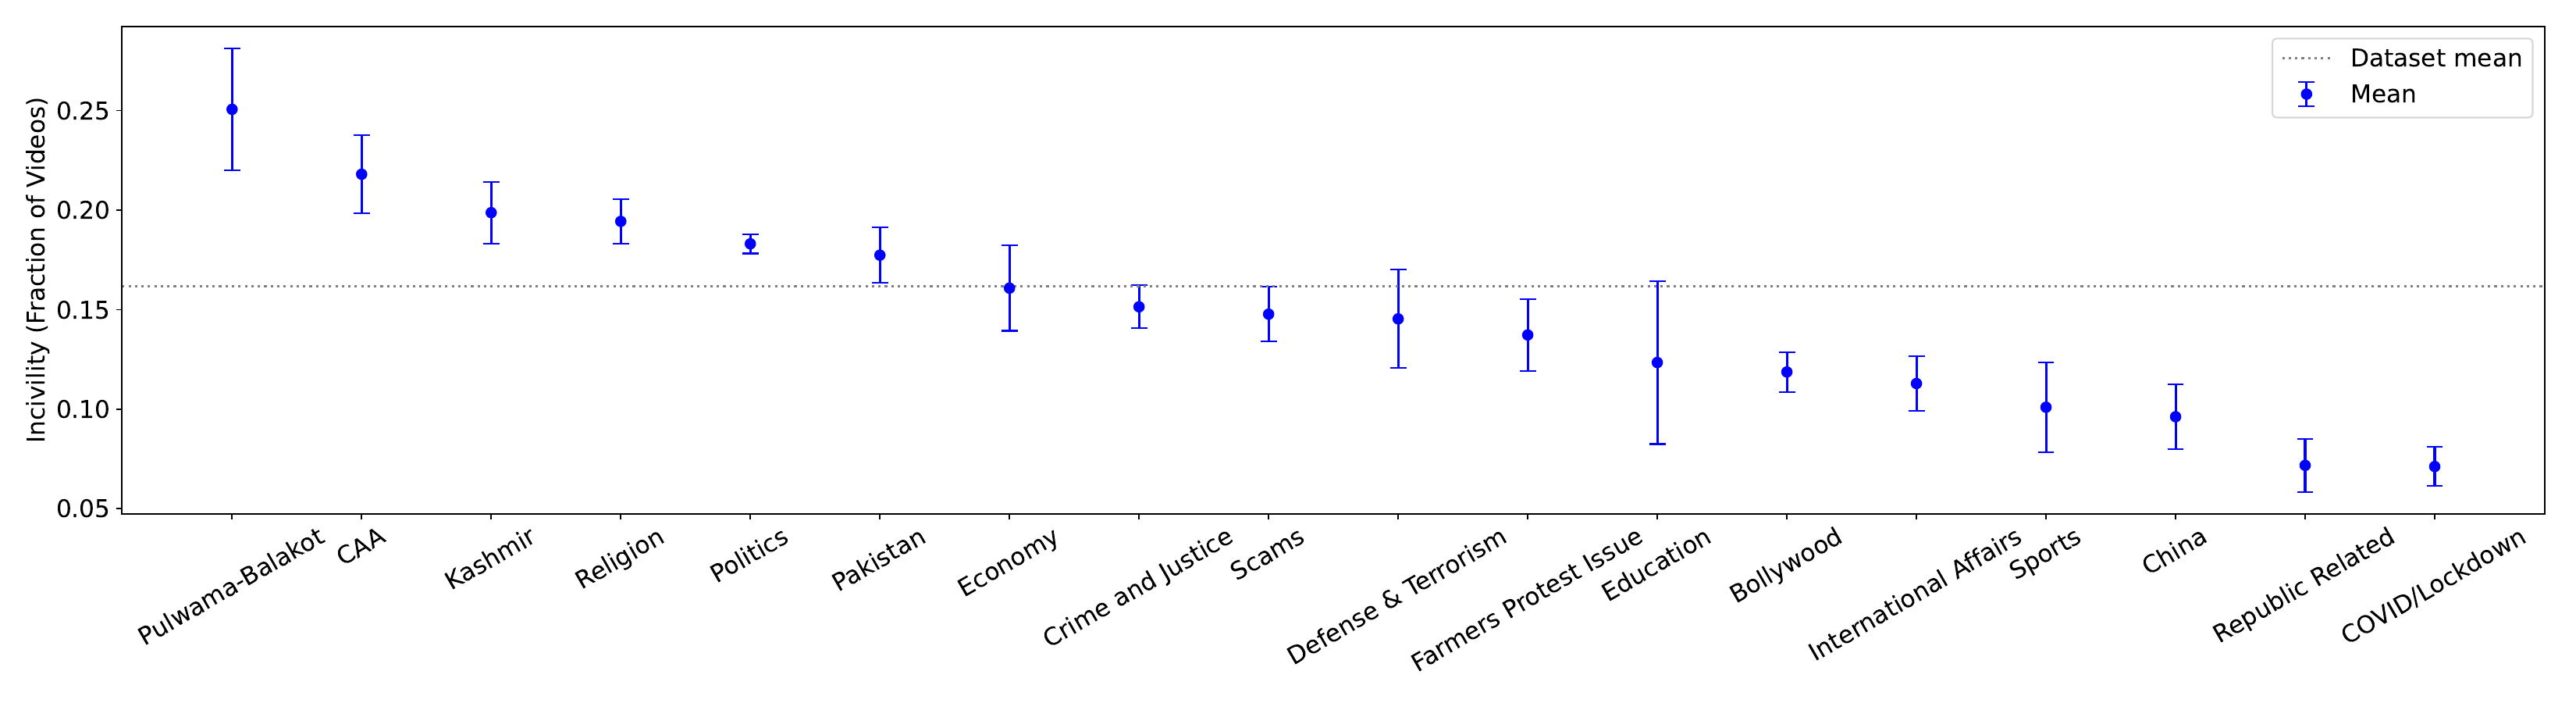}
  \caption{Incivility for all categories.}
  \label{fig:incivility_all}
\end{figure*}

\begin{figure*}[htbp]
  \centering
  \includegraphics[width=1\linewidth]{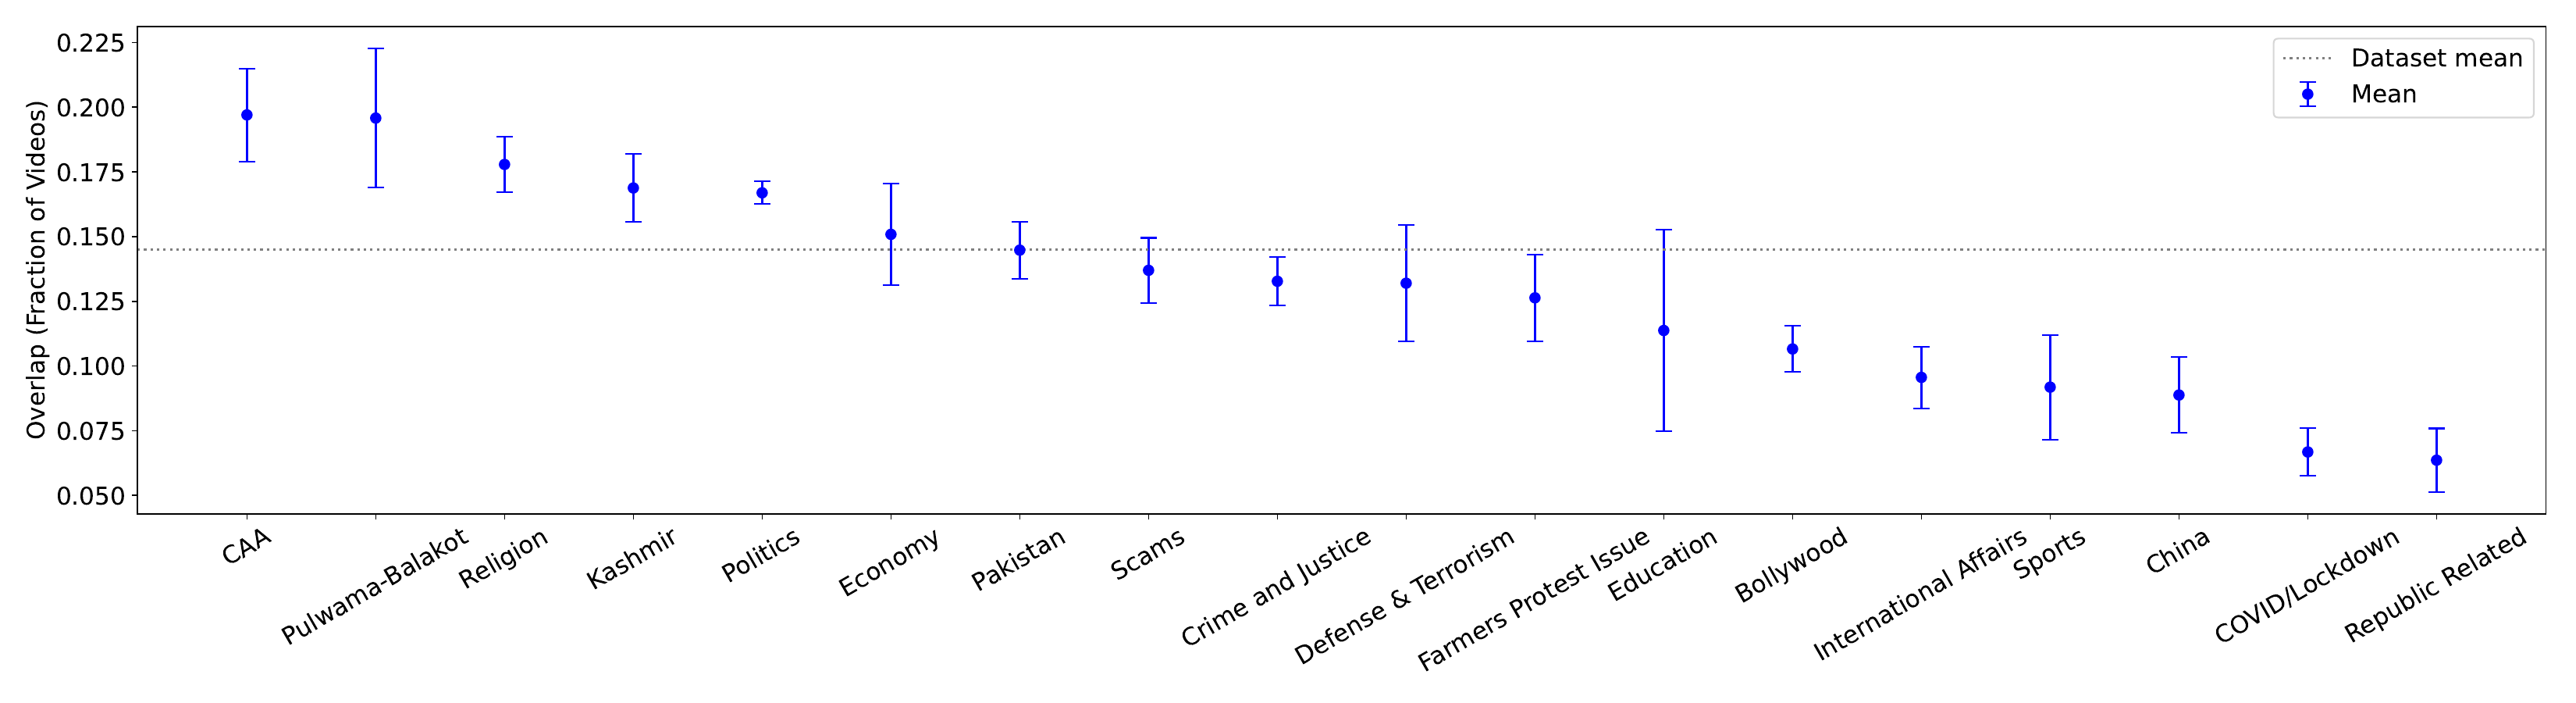}
  \caption{Overlap speech for all categories.}
  \label{fig:overlap_all}
\end{figure*}

\begin{figure}
  \centering
  \includegraphics[width=1\linewidth]{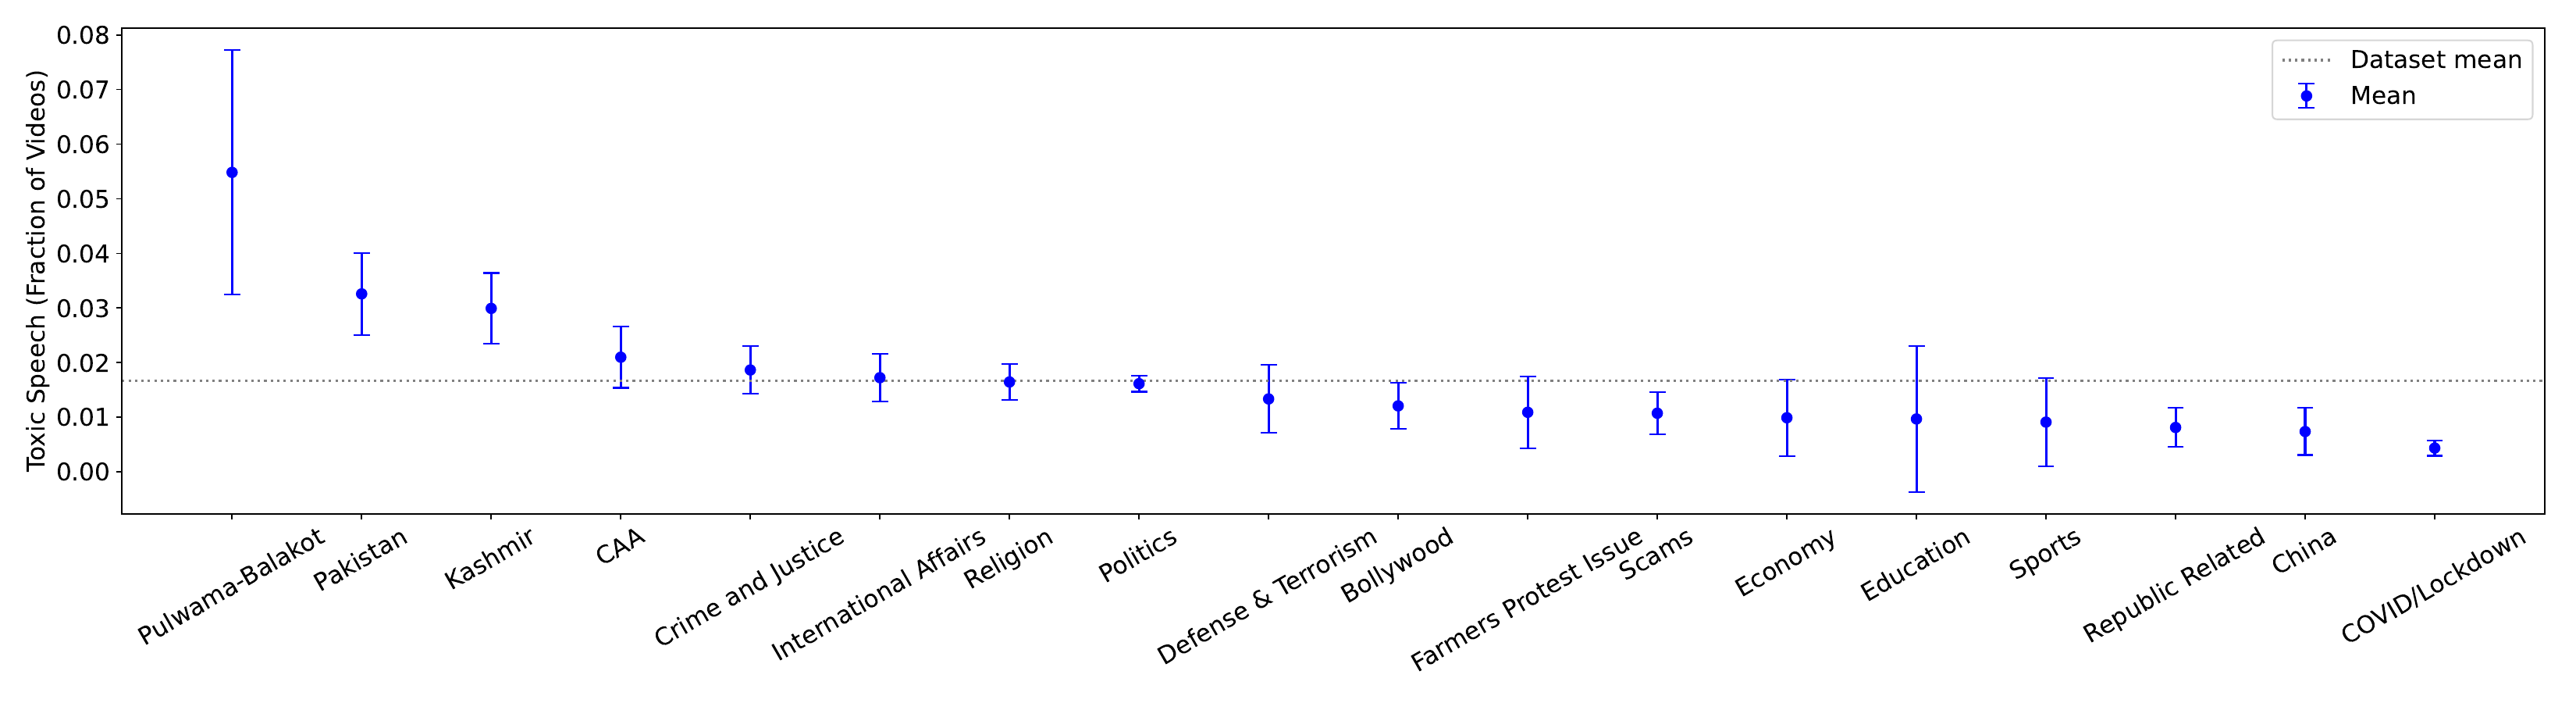}
  \caption{Fraction of videos with toxic speech in all categories}
  \label{fig:toxic_all}
    \end{figure}

\begin{figure*}[htbp]

\end{figure*}

\begin{figure*}[htbp]
  \centering
  \includegraphics[width=1\linewidth]{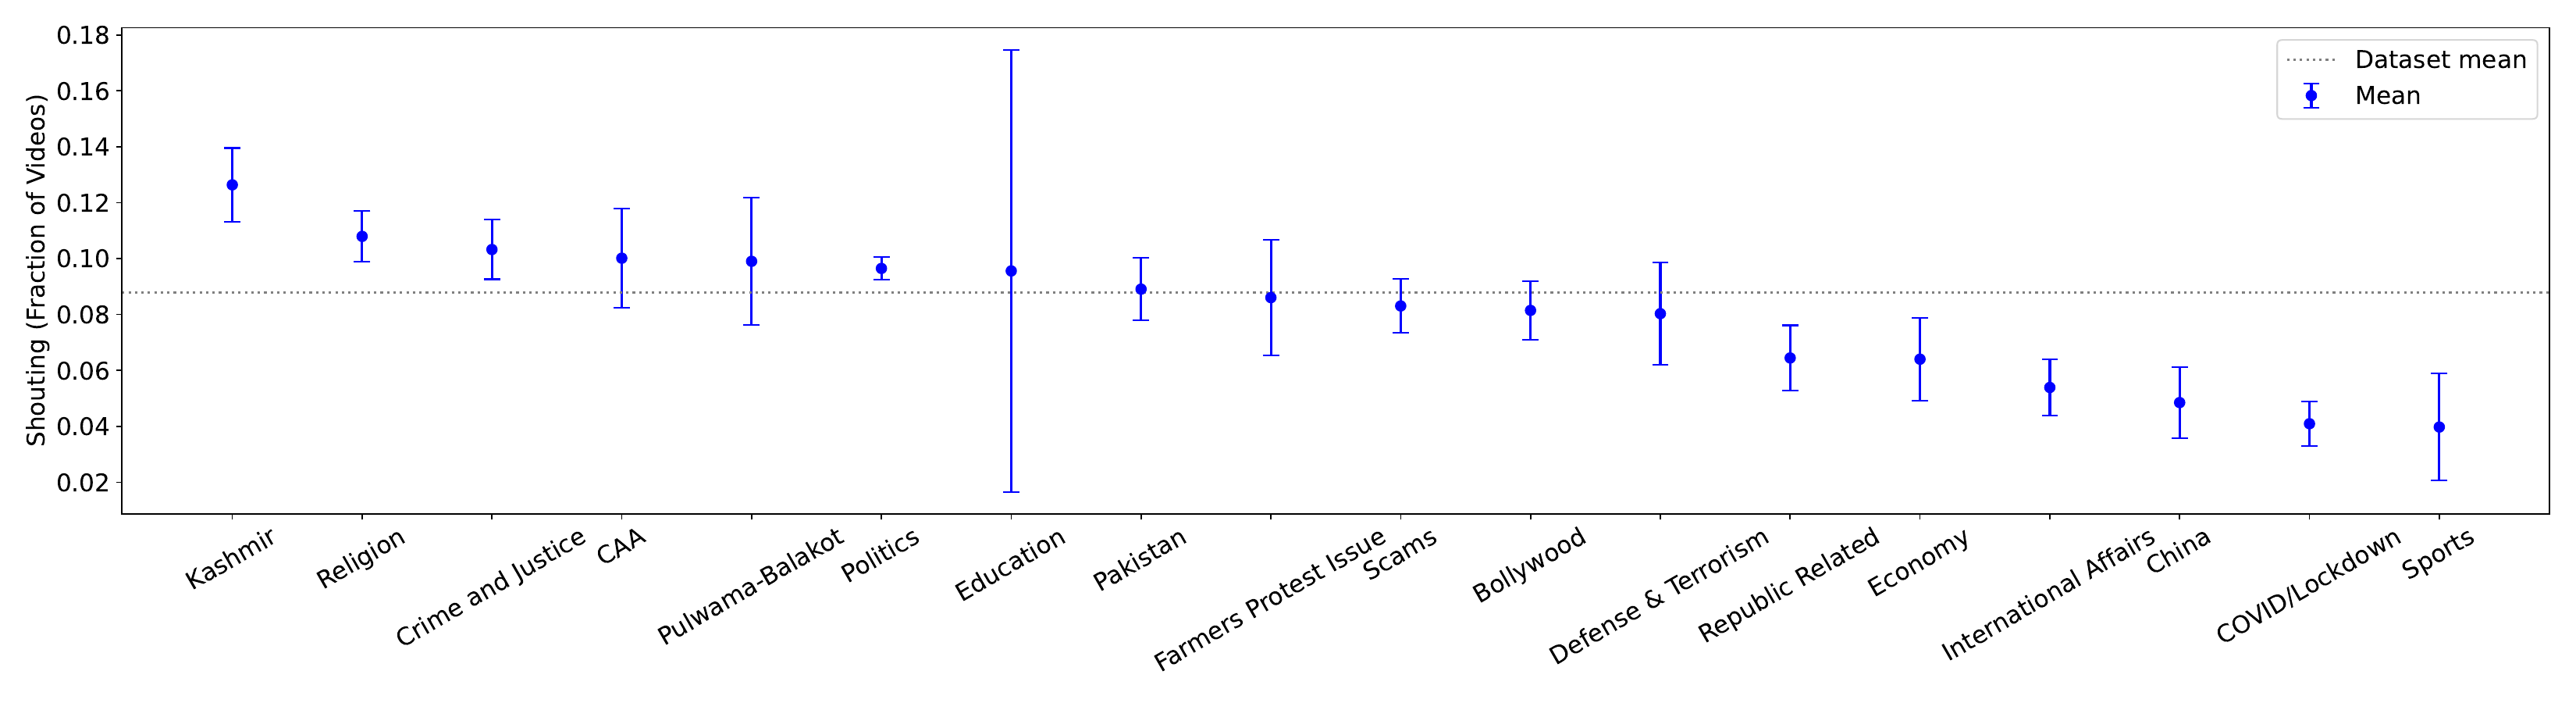}
  \caption{Fraction of videos with shouting in all categories}
  \label{fig:shouting_frac_ci_appendix}
\end{figure*}

\begin{figure*}[htbp]
  \centering
  \includegraphics[width=1\linewidth]{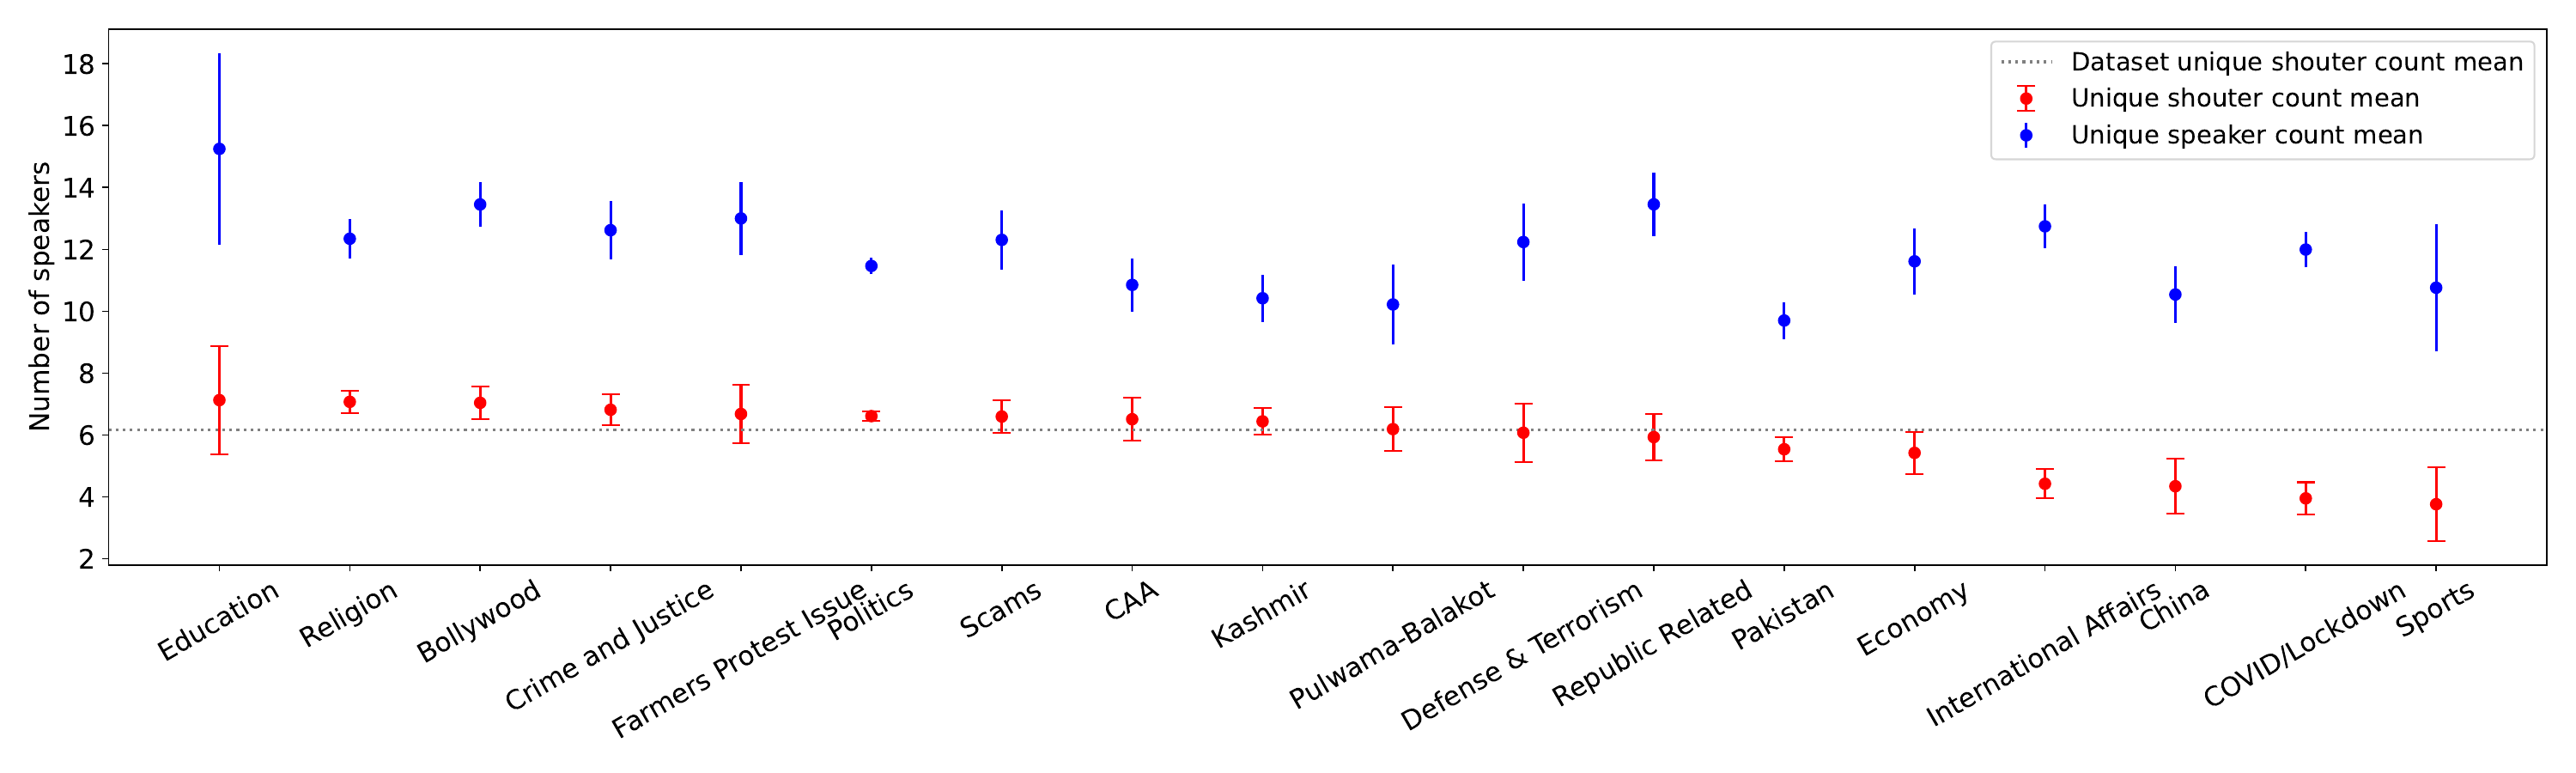}
  \caption{Number of unique shouters per video in all categories}
\end{figure*}

\subsection{Gender Bias}

Figure \ref{fig:female_size_lesser_males} shows the trends in the average screen real estate allocated to male and female faces over the years. We can clearly see that there is a significant gap --- even if a woman is present on the screen, they are not given enough space.

\begin{figure}
        \centering
        \includegraphics[width=1\linewidth, clip=true, trim=0 25 0 10]{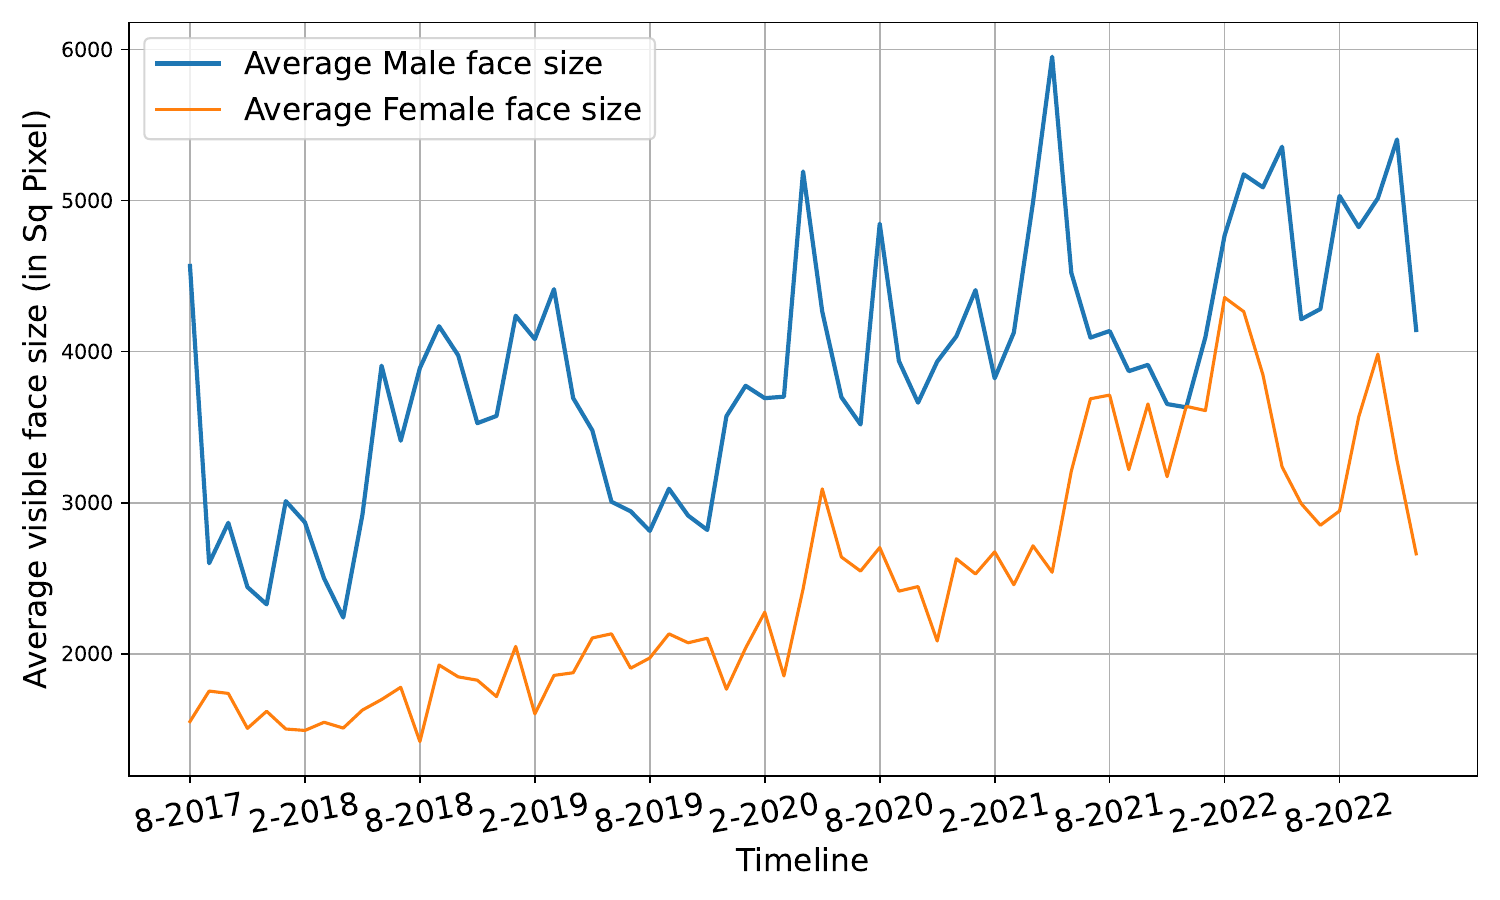}
        \caption{Average size of faces (Males: 3798 sq pixels, Females: 2424 pixels)}
        \label{fig:female_size_lesser_males}
        %\vspace{-\baselineskip}
\end{figure}

Figure \ref{fig:female_faces_full} shows the fraction videos with female faces in all categories.

\begin{figure*}[htbp]
  \centering
  \includegraphics[width=1\linewidth]{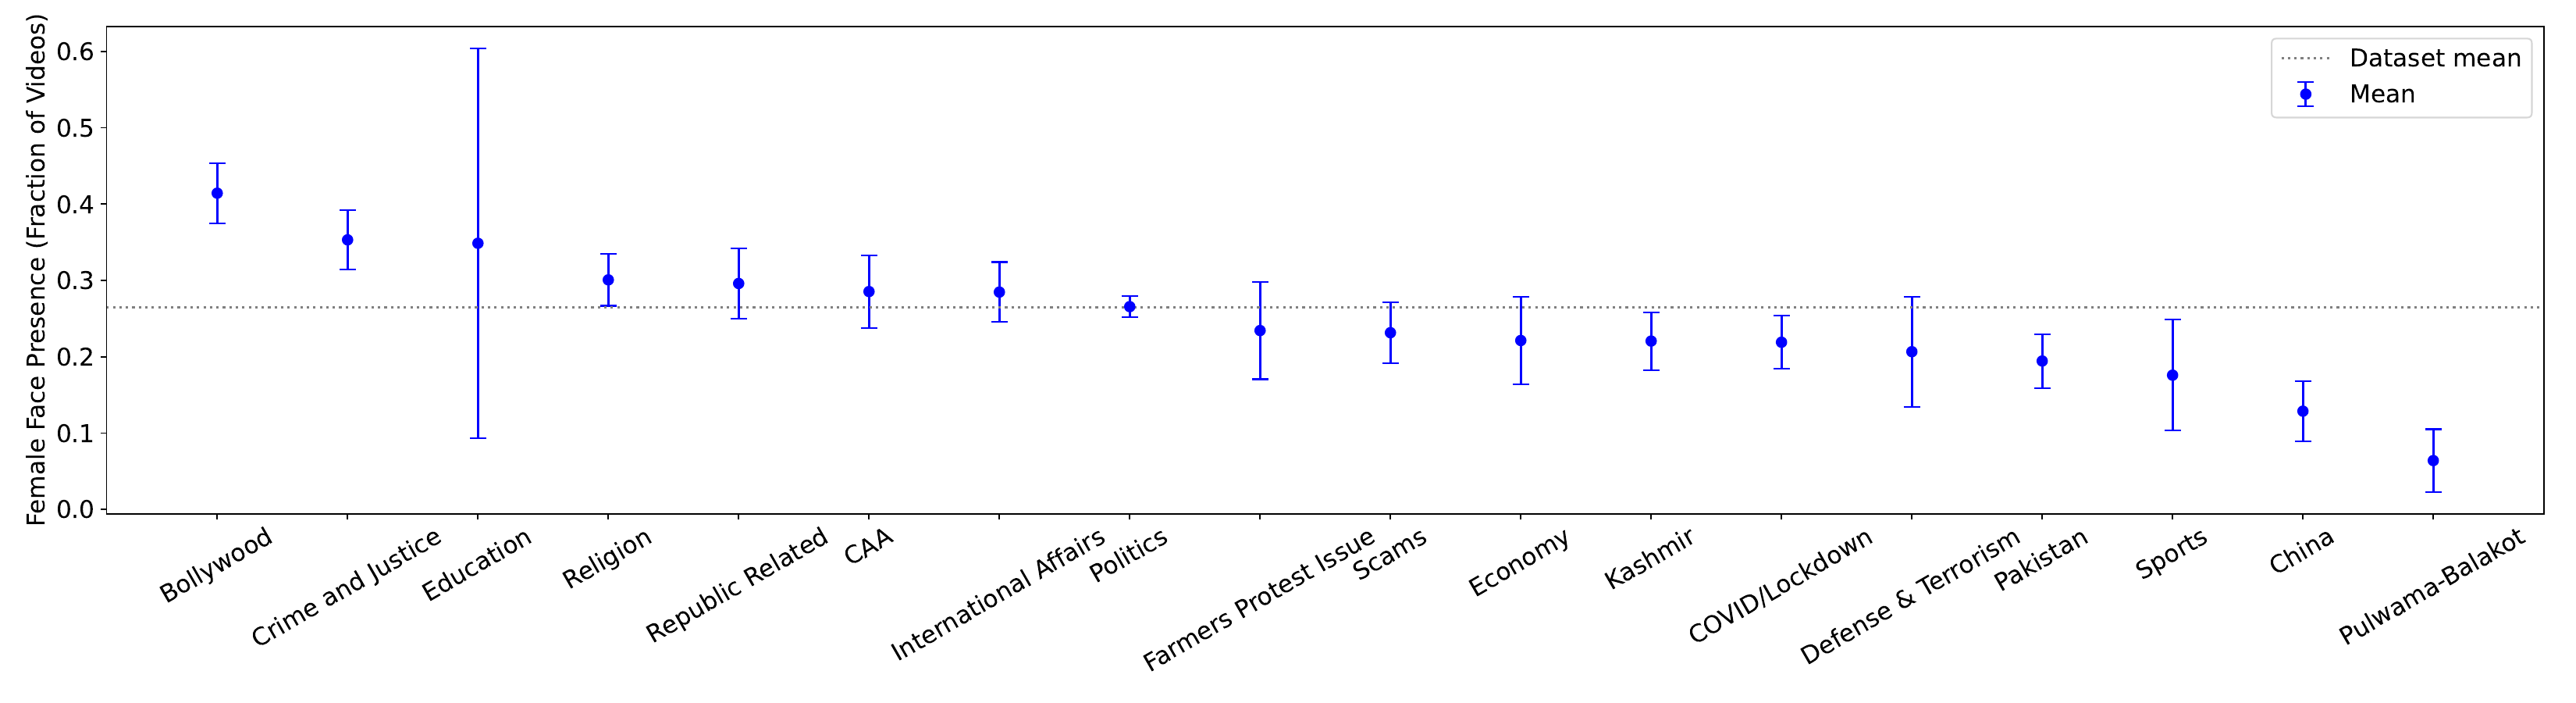}
  \caption{Fraction of videos with female faces in all categories}
  \label{fig:female_faces_full}
\end{figure*}

\subsection{Network analysis of panelists}

\begin{figure*}
        \centering
        \includegraphics[width=0.9\linewidth]{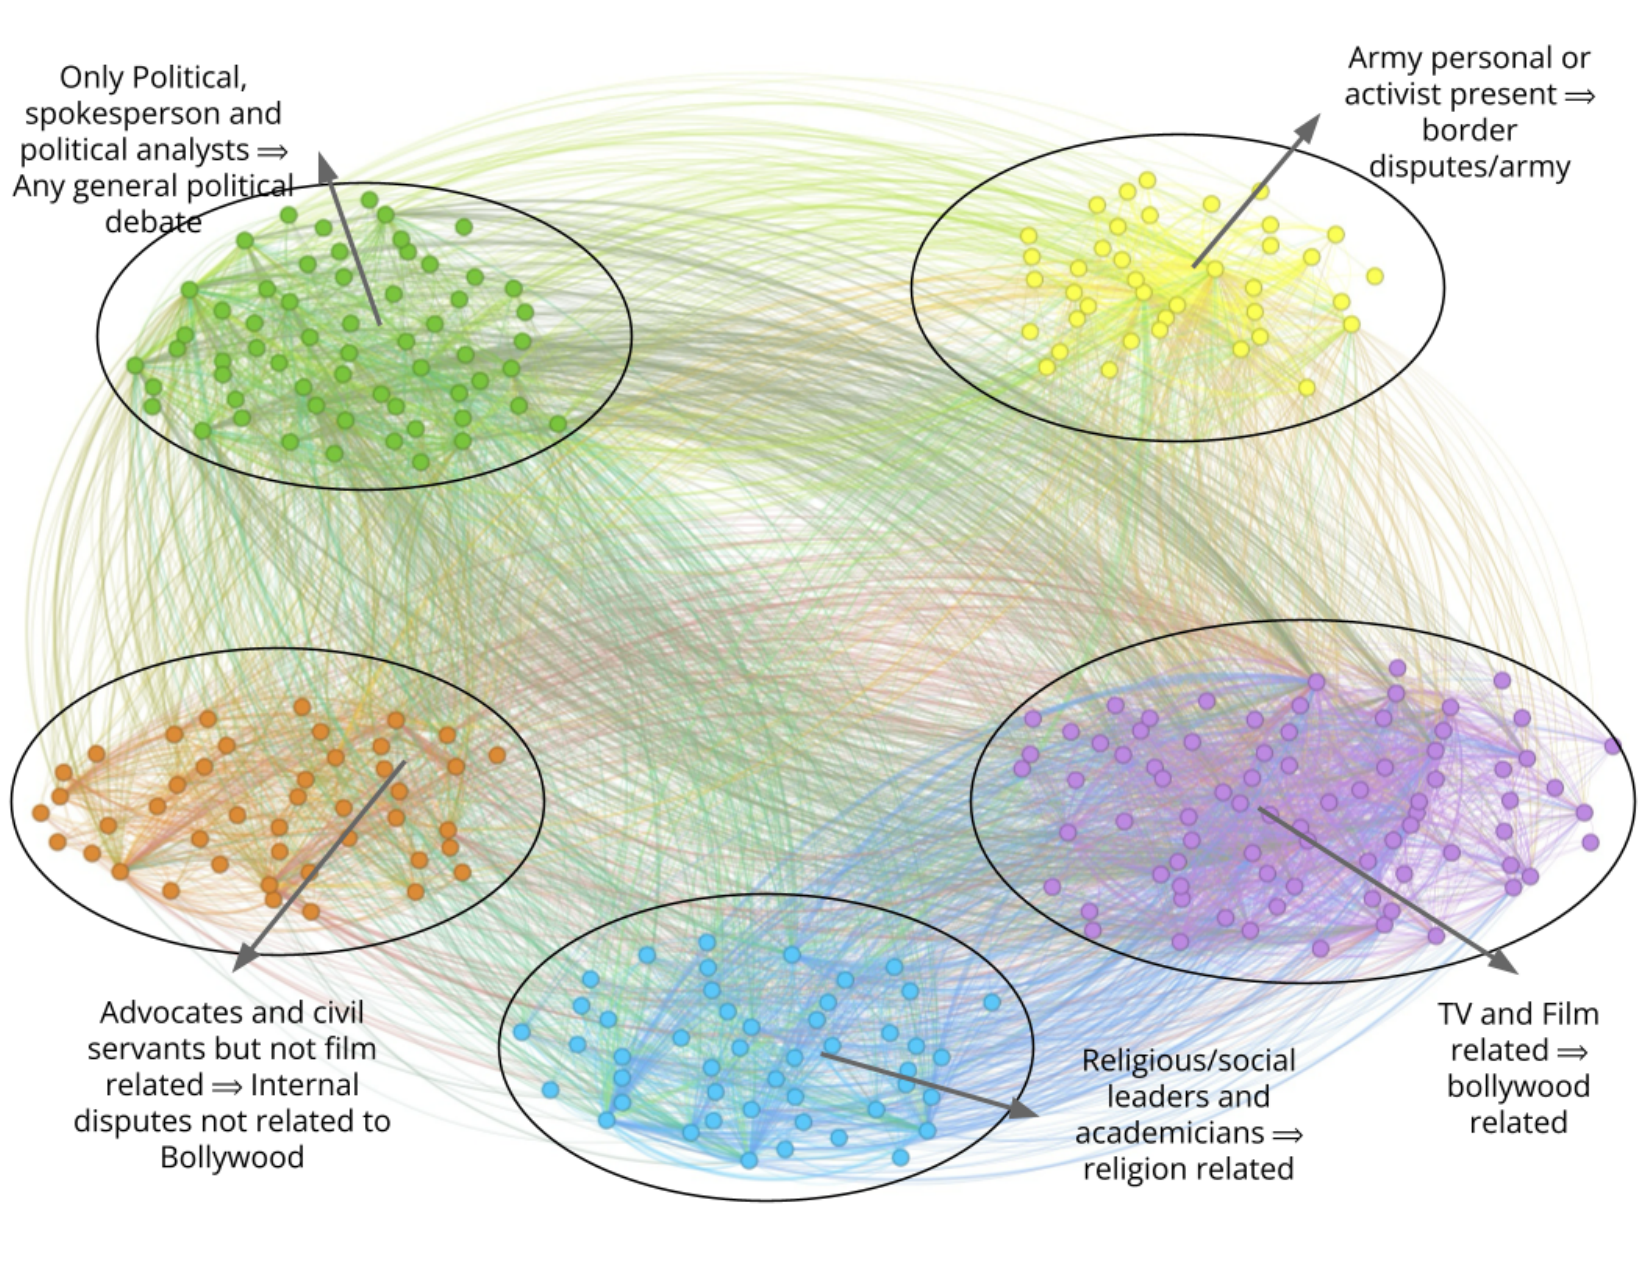}
        \caption{Found five kinds of clusters inside people affiliation coming on debate.}
        \label{fig:network_affiliation}
\end{figure*}
\label{sec:appendix_shouting1}
Using the information of the panelists we manually coded in Section \ref{sec:panelist_names}, we created a co-occurrence network between the panelists. If two panelists appeared together in a debate, they were connected by an edge.
Perhaps not so surprisingly, with just this information, we found that such a network (shown in Figure \ref{fig:network_affiliation}) 
was clearly clustered along categories and occupations of the panelists, indicating that the show invites specific panelists based on specific topics of discussion over and over. The five communities were automatically identified using the Louvain method for community detection and correspond to topics like General politics, Religion, Bollywood, and Army related issues.  
%\kiran{how were these communities identified? Using Gephi's community detection algorithm (Louvain method)} 
%Though this clustering is not surprising...
%Figure \ref{fig:network_affiliation} \\
\begin{enumerate}
    \item Orange: Found occupation like Advocate, civil servants but not film related occupation $\rightarrow$ Not related to Bollywood internal disputes 
    \item Blue: All religious/social leaders and academic people $\rightarrow$ Something related to religion 
    \item Pink: All TV and film related people $\rightarrow$ related to Bollywood
    \item Yellow: Army related personal, activists $\rightarrow$ related to border disputes/army
    \item Green: Only politician, spokesperson and analyst $\rightarrow$ Any general political debate
\end{enumerate}

\begin{table}[h]
    \centering
     \caption{Affiliation Triads with a statistically significant difference in incivility compared to overall incivility. Incivility values here are the sum of overlap and toxicity.}
    \label{tab:triad_incivility}
    \begin{tabular}{|p{0.3\columnwidth}|p{0.3\columnwidth}|p{0.3\columnwidth}|}
    \hline
    Triad & Average incivility fraction in videos where they occur & Frequency of them occurring in a video \\ 
    \hline
    DMK-BJP-BJP & 0.218 & 72 \\
    \hline
    Congress-BJP-AAP & 0.209 & 52 \\
    \hline
    BJP-AAP-BJP & 0.204 & 88 \\
    \hline
    BJP-Samajwadi party-BJP & 0.189 & 70 \\
    \hline
    TMC-BJP-BJP & 0.179 & 148 \\
    
    \hline
    \end{tabular}
\end{table}

\subsection{Incivility based on participants}
\label{sec:incivility_participants}
In our analysis, we delved into the relationship between panelist participation and the level of incivility in the debates. Specifically, we were interested in understanding whether the presence of certain types of panelists could be linked to increased incivility. To examine this, we utilized the annotations identifying each panelist's political party affiliation. We focused on key opposition parties, such as Congress, All India Trinamool Congress (TMC), Aam Aadmi Party (AAP), DMK, and the Samajwadi Party, to create triads of participants for each video. In these triads, at least one member was affiliated with the ruling party, and the remaining two were from opposition parties, or vice versa.

To ensure robust findings, we filtered out triads that occurred less than 50 times across all videos. We then calculated the average incivility for videos featuring these triads and found that the incivility was statistically higher (p<0.05) than the dataset's overall average incivility of 0.162. Notably, the triads comprising panelists from opposition parties were associated with higher levels of incivility. Table \ref{tab:triad_incivility} shows the results.

These results suggest that the composition of the panel, particularly the presence of opposition party representatives, may be a significant factor in driving incivility in these debates. This raises questions about the dynamics at play during the debates and how they may be influenced by the panelists' political affiliations. It suggests a need for further scrutiny into whether the heightened incivility is a result of the topics being discussed, the panelists' tactics, or perhaps editorial choices.
